# Supplementary material for: Optomechanical microwave amplification without mechanical amplification
Source: arXiv:1812.05459 ancillary file (2020-01-22)
Supplement: Supplementary file 1 [file omit_amp_si_v0.6.pdf]

# **Supplementary Material: Optomechanical microwave amplification without mechanical amplification**

Martijn A. Cohen\*, Daniel Bothner\*, Yaroslav M. Blanter, and Gary A. Steele

*Kavli Institute of Nanoscience, Delft University  
of Technology, 2628 CJ Delft, The Netherlands*

(Dated: December 13, 2018)

## S1. FABRICATION

We fabricated the antenna chip and membrane chip separately. The antenna chip was made from double-side polished sapphire 420  $\mu\text{m}$  thick and it was pre-cleaned using a Piranha solution –  $\text{H}_2\text{SO}_4$  and  $\text{H}_2\text{O}_2$  in (3:1) concentration, heated to 80° C for roughly 10 minutes. We sputter-deposited 100 nm of Molybdenum-Rhenium alloy (MoRe 60/40) and spun AZ ECI 3007 photoresist. The antennas were patterned using a Durham Magneto Optics Microwriter ML-2 laserwriter and the remaining MoRe was then etched away using an  $\text{SF}_6/\text{He}$  plasma. The photoresist was stripped using warm N-Methyl-2-pyrrolidone (NMP).

The membrane chip was metalized using a lift-off method because we had adhesion issues when spinning photoresist onto a MoRe-coated membrane as seen in Fig. S1(a). The photoresist would crack off which we believe is because the membrane was an unstable surface which could move when the photoresist would be developed. We patterned using a negative photoresist – AZ 5214E – and sputtered 20 nm of MoRe. We made sure that the patch overlapped with the frame of the Norcada membrane to induce mechanical losses and increase the amplification bandwidth<sup>S1</sup>. The lift-off procedure was then also performed using warm NMP.

We flipped the two chips on top of each other and fixed them by using a small drop of epoxy on the corner of the membrane chip. We would wait an hour until we were sure the drop of glue was healed.

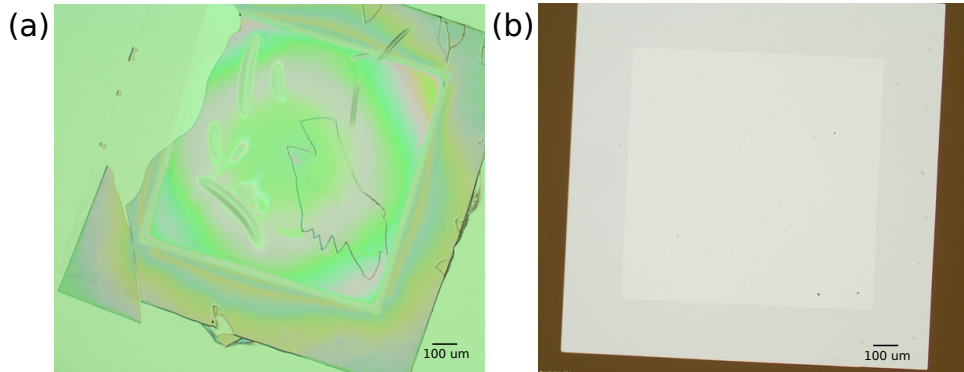

FIG. S1. (a) An optical micrograph of photoresist failing to adhere to the MoRe-coated Norcada membrane. (b) here the MoRe patch can be seen overlapping with the frame using a lift-off method.

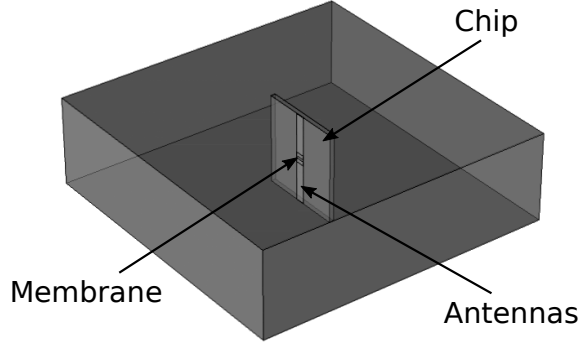

FIG. S2. A figure showing the geometry of our COMSOL simulation. The chip in the middle contains two antennas and a membrane in the center which approximates our capacitive circuit. The gap of the membrane is modulated to calculate the coupling constant.

## S2. ESTIMATING COUPLING CONSTANT

We estimate the optomechanical coupling constant using finite element model simulations in COMSOL. We recreate the geometry of our chip by including a sapphire chip with a thickness of  $430\text{ }\mu\text{m}$ , on top of which we patterned our antennas. In between the arms of the antennas we put a  $1 \times 1\text{ mm}$  metal square which corresponds to the metalized membrane, as sketch of which can be seen in Fig. S2. Even though the geometry of the capacitance between the antennas and cavity walls is different in the COMSOL model due to computational ease, we compensate for this by decreasing the gap between the antennas and the wall such that the resonance frequency of the entire structure matches what we measured empirically. We can use the following formula to derive the coupling constant

$$g_0 = \frac{d\omega_0}{dx} x_{\text{zpf}} \quad (\text{S1})$$

where  $\frac{d\omega_0}{dx}$  is the rate of change of the cavity resonance frequency with respect to the membrane gap.  $x_{\text{zpf}}$  corresponds to the zero point fluctuations of the mechanical oscillator and can be calculated by  $x_{\text{zpf}} = \sqrt{\frac{\hbar}{2m\Omega_m}}$  which for our MoRe-coated membrane is  $0.28\text{ fm}$ . We determine the rate of change of the cavity by simulating the resonance at two points around the estimated membrane gap of  $2\text{ }\mu\text{m}$  and arrive at  $\frac{d\omega_0}{dx} \approx 246\text{ kHz/nm}$ . This results in a coupling strength  $g_0/2\pi \approx 0.069\text{ Hz}$ .

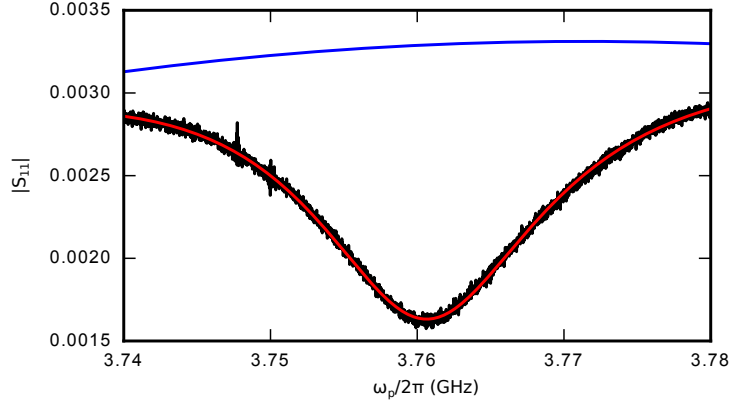

FIG. S3. A reflection measurement of the cavity response in linear units. The data in black is the raw signal, blue signifies the background fit, and red is the total fit.

### S3. NORMALIZATION OF BACKGROUND SIGNAL

Before we fit and extract data from the reflection measurement, we have to fit the background signal. For this we use a complex polynomial as an approximation

$$S_{11,b}(\omega) = (a + b\omega + c\omega^2)e^{i(a'+b'\omega)} \quad (\text{S2})$$

where all variables except  $\omega$  are fitting constants. When fitting the full cavity response we first extract the resonance frequency and eliminate it from the data. We then make a preliminary fit of this modified data. Using the fit parameters for the complex polynomial above, we then refit the raw data using both the background and a Lorentzian for the cavity response using the following formula

$$S_{11}(\omega) = S_{11,b}(\omega) \times \left( \frac{2\kappa_e e^{i\theta}}{\kappa_e + \kappa_i - 2i(\omega - \omega_0)} - 1 \right) \quad (\text{S3})$$

where, again, all variables except  $\omega$  are fitting constants. Figure S3 shows the raw data with both fits.

#### S4. DERIVATION OF FULL EQUATIONS OF MOTION

We start by citing the classical optomechanical equations of motion as derived throughout literature in the field of optomechanics<sup>S2,S3</sup>

$$\ddot{x} = -\Omega_m^2 x - \Gamma_m \dot{x} + \frac{\hbar G}{m} |\alpha|^2 \quad (\text{S4})$$

$$\dot{\alpha} = i(\Delta + Gx)\alpha - \frac{\kappa}{2}\alpha + \sqrt{\kappa_e} s_{\text{in}} \quad (\text{S5})$$

The first equation describes the displacement  $x$  of the mechanical oscillator, the second describes the intracavity field amplitude  $\alpha$ . In the first equation,  $\Omega_m$  is the resonance frequency of the mechanical oscillator,  $\Gamma_m$  is the mechanical damping rate and  $m$  is the effective mass of the mechanical oscillator. The last term is the radiation pressure force, where  $G = -\partial\omega_0/\partial x$  is the cavity pull parameter. In the second equation the light field amplitude  $\alpha$  is normalized such that  $|\alpha|^2$  is the photon number in the cavity,  $\Delta = \omega_d - \omega_0$  denotes the detuning between the drive frequency  $\omega_d$  and the cavity resonance frequency  $\omega_0$ .  $\kappa$  is the total cavity linewidth and  $\kappa_e$  is the external coupling constant.  $s_{\text{in}}$  is an input drive signal.

We assume now that a static equilibrium solution exists with  $\dot{x} = \dot{\alpha} = 0$  and  $x = \bar{x}$  and  $\alpha = \bar{\alpha}$ . We find from the equations of motion

$$\bar{x} = \frac{\hbar G}{m\Omega_m^2} |\bar{\alpha}|^2 \quad (\text{S6})$$

$$\bar{\alpha} = s_{\text{in}} \frac{\sqrt{\kappa_e}}{\frac{\kappa}{2} - i\bar{\Delta}} \quad (\text{S7})$$

where  $\bar{\Delta} = \omega_d - \omega_0 + G\bar{x}$ . (Note that in the main text we simplify by using  $\Delta$  when in reality we mean  $\bar{\Delta}$ .) Secondly, we assume that it is sufficient to consider small deviations from this equilibrium solution and set  $\alpha = \bar{\alpha} + \delta\alpha$  and  $x = \bar{x} + \delta x$ . We linearize the equations of motion and throw away quadratic terms in  $\delta x$  and  $\delta\alpha$ . We arrive at the two coupled, linearized equations

$$\delta\ddot{x} = -\Omega_m^2 \delta x - \Gamma_m \delta\dot{x} + \frac{\hbar G \bar{\alpha}}{m} (\delta\alpha + \delta\alpha^*) \quad (\text{S8})$$

$$\delta\dot{\alpha} = \left[ i\bar{\Delta} - \frac{\kappa}{2} \right] \delta\alpha + iG\bar{\alpha}\delta x + \sqrt{\kappa_e} s_p \quad (\text{S9})$$

where we assume that  $\bar{\alpha}$  is real and where the last term accounts for small additional probe fields  $s_p = s_0 e^{-i\Omega t}$  with the difference between the probe and drive frequency  $\Omega = \omega_p - \omega_d$  in the frame rotating with  $\omega_d$ .

To solve the equations, we use the ansatz

$$\delta\alpha = a_- e^{-i\Omega t} + a_+ e^{+i\Omega t} \quad (\text{S10})$$

$$\delta\alpha^* = a_-^* e^{+i\Omega t} + a_+^* e^{-i\Omega t} \quad (\text{S11})$$

$$\delta x = x_1 e^{-i\Omega t} + x_1^* e^{+i\Omega t} \quad (\text{S12})$$

and we keep only the terms resonant with the drive  $\propto e^{-i\Omega t}$ .

We get three equations

$$x_1[\Omega_m^2 - \Omega^2 - i\Omega\Gamma_m] = \frac{\hbar G \bar{\alpha}}{m} (a_- + a_+^*) \quad (\text{S13})$$

$$a_- \left[ \frac{\kappa}{2} - i(\bar{\Delta} + \Omega) \right] = iG\bar{\alpha}x_1 + \sqrt{\kappa_e} s_0 \quad (\text{S14})$$

$$a_+^* \left[ \frac{\kappa}{2} + i(\bar{\Delta} - \Omega) \right] = -iG\bar{\alpha}x_1 \quad (\text{S15})$$

Next, we remove  $a_+^*$  and  $x_1$  from the first equation with the second and third and get for  $a_-$  the expression

$$a_- = \frac{1 + if(\Omega)}{\kappa/2 - i(\bar{\Delta} + \Omega) + 2\bar{\Delta}f(\Omega)} \sqrt{\kappa_e} s_0 \quad (\text{S16})$$

with

$$f(\Omega) = \frac{\hbar G^2 \bar{\alpha}^2}{\kappa/2 + i(\bar{\Delta} - \Omega)} \chi_m(\Omega) \quad (\text{S17})$$

and the mechanical susceptibility

$$\chi_m(\Omega) = \frac{1}{m(\Omega_m^2 - \Omega^2 - i\Omega\Gamma_m)} \quad (\text{S18})$$

We can use input-output theory to use these equations to calculate a reflection coefficient at a single port cavity:

$$S_{11} = 1 - \sqrt{\kappa_e} \frac{a_-}{s_0} \quad (\text{S19})$$

We calculate the reflection coefficient when there is no dynamical backaction by setting the drive tone resonant with the cavity frequency  $\bar{\Delta} = 0$  and the probe detuning to negative and positive the mechanical frequency  $\Omega = \pm\Omega_m$

$$S_{11}(\bar{\Delta} = 0, \Omega = \pm\Omega_m) = 1 - \frac{\kappa_e}{\kappa/2 \mp i\Omega_m} \pm C \frac{\kappa\kappa_e/2}{(\kappa/2 \mp i\Omega_m)^2} \quad (\text{S20})$$

where  $C = \frac{4g_0^2}{\Gamma_m \kappa} n_d$  is the multi-photon cooperativity. The first two terms are the typical cavity response function, while the last term is purely due to optomechanical interactions.

We can further simplify by assuming we are deeply sideband-unresolved ( $\kappa \gg \Omega_m$ ) and using  $\eta = \kappa_e/\kappa$

$$S_{11}(\pm\Omega_m) = 1 - 2\eta \pm 2\eta C = 1 - 2\eta(1 \mp C) \quad (\text{S21})$$

which exceeds 1 in the limit  $C \gg 1$ , indicating amplification.

## S5. DERIVATION OF MIXING PICTURE

We can derive Eq. (S20) in a slightly different way to give more insight as to why this amplification occurs. Starting with mechanical displacement, we will do this in four steps.

### 1. Mechanical displacement

The radiation pressure force onto the mechanical oscillator due to an intracavity field is given by

$$F_r = \hbar G |\alpha|^2. \quad (\text{S22})$$

Assuming again that the intracavity field can be approximated by  $\alpha = \bar{\alpha} + \delta\alpha$  with constant  $\bar{\alpha}$  this reads

$$F_r \approx \hbar G |\bar{\alpha}|^2 + \hbar G (\bar{\alpha}^* \delta\alpha + \bar{\alpha} \delta\alpha^*) \quad (\text{S23})$$

where we once again omitted the term  $\propto |\delta\alpha|^2$ .

We get the mechanical displacement  $\delta x = x - \bar{x}$  for a driving frequency  $\Omega = \pm\Omega_m$  from here by using the mechanical susceptibility Eq. (S18) as

$$\delta x = \pm i \hbar G \frac{\bar{\alpha}^* \delta\alpha + \bar{\alpha} \delta\alpha^*}{m\Omega_m \Gamma_m} \quad (\text{S24})$$

or for a real-valued average amplitude  $\bar{\alpha}$

$$\delta x = \pm i \frac{\hbar G \bar{\alpha}}{m\Omega_m \Gamma_m} (\delta\alpha + \delta\alpha^*) \quad (\text{S25})$$

## 2. Exciting the mechanical oscillator

Next, we assume that we drive the cavity with a strong microwave tone  $s_{\text{in}}$  on resonance  $\bar{\Delta} = 0$  and with a much smaller probe tone  $s_0$  one mechanical frequency detuned from it  $\Omega = \pm\Omega_{\text{m}}$ . The intracavity field to first order is then given by

$$\bar{\alpha} + \delta\alpha = 2\frac{\sqrt{\kappa_{\text{e}}}}{\kappa}s_{\text{in}} + \frac{\sqrt{\kappa_{\text{e}}}}{\kappa/2 \mp i\Omega_{\text{m}}}s_0e^{\mp i\Omega_{\text{m}}t}. \quad (\text{S26})$$

and the term relevant for the radiation pressure force by

$$\delta\alpha + \delta\alpha^* = \frac{\sqrt{\kappa_{\text{e}}}}{\kappa/2 \mp i\Omega_{\text{m}}}s_0e^{\mp i\Omega_{\text{m}}t} + \frac{\sqrt{\kappa_{\text{e}}}}{\kappa/2 \pm i\Omega_{\text{m}}}s_0e^{\pm i\Omega_{\text{m}}t} \quad (\text{S27})$$

We implicitly assumed here that  $s_0$  is real-valued, fixing the phase between  $s_{\text{in}}$  and  $s_0$  at  $t = 0$ .

From here, we can calculate  $x_1$  and  $x_2$  of  $\delta x = x_1e^{-i\Omega_{\text{m}}t} + x_2e^{+i\Omega_{\text{m}}t}$  as

$$x_1 = \pm i \frac{\hbar G \bar{\alpha}}{m\Omega_{\text{m}}\Gamma_{\text{m}}} \frac{\sqrt{\kappa_{\text{e}}}}{\kappa/2 \mp i\Omega_{\text{m}}} s_0 \quad (\text{S28})$$

$$x_2 = \pm i \frac{\hbar G \bar{\alpha}}{m\Omega_{\text{m}}\Gamma_{\text{m}}} \frac{\sqrt{\kappa_{\text{e}}}}{\kappa/2 \pm i\Omega_{\text{m}}} s_0 \quad (\text{S29})$$

We note, that in this choice of phases we get  $\delta x(+\Omega_{\text{m}}) = -\delta x(-\Omega_{\text{m}})$ , i.e., for blue vs red detuned probe tone the mechanical oscillations are shifted by  $\pi$  with respect to each other. Also, due to fixing the phase of  $s_0$  above, we cannot use the general approach  $\delta x = x_1e^{-i\Omega_{\text{m}}t} + x_1^*e^{+i\Omega_{\text{m}}t}$  as we have to allow for an additional phase shift. Here, we get as result  $x_2 = -x_1^*$ .

## 3. Drive sideband generation

Now we assume the cavity is driven on resonance  $\bar{\Delta} = 0$  with a single tone and that the mechanical resonator is oscillating with  $\delta x(t) = x_1e^{-i\Omega_{\text{m}}t} - x_1^*e^{+i\Omega_{\text{m}}t}$ . From Eq. (S14), we get for this case

$$a_{s-} = iG \frac{\bar{\alpha}}{\kappa/2 - i\Omega_{\text{m}}} x_1 \quad (\text{S30})$$

$$a_{s+} = -iG \frac{\bar{\alpha}}{\kappa/2 + i\Omega_{\text{m}}} x_1^*. \quad (\text{S31})$$

These two amplitudes correspond to the two sidebands to the resonant drive tone, which are generated by the mechanical motion. One sideband with amplitude  $a_{s+}$  is oscillating at  $\omega_0 + \Omega_m$  and one with amplitude  $a_{s-}$  at  $\omega_0 - \Omega_m$ , cf. Eq. (S10). As can be derived from the expressions, there is also a phase-shift of  $\pi$  between them, which means that  $\delta\alpha_s + \delta\alpha_s^* = 0$  with  $\delta\alpha_s = a_{s-}e^{-i\Omega_m t} + a_{s+}e^{+i\Omega_m t}$ , i.e., that there is no dynamical backaction acting upon the mechanical oscillator when only considering a resonant drive and those two sidebands, cf. Eq. (S8).

#### 4. Amplification for $\Omega = +\Omega_m$

Finally, we put the ingredients together. The mechanical oscillator is driven into a motional state with amplitude  $\delta x$  by a combination of a drive tone resonant with the cavity and a probe tone one mechanical frequency detuned. The resulting motion modulates the cavity frequency and generates sidebands to the drive tone, one of which interferes with the probe tone. The intracavity field at this frequency is then given by the interference of the probe tone amplitude and the sideband of the drive

$$a_- = \delta\alpha + a_{s-} = \frac{\sqrt{\kappa_e}}{\kappa/2 - i\Omega_m} s_0 - \frac{\kappa}{2} C \frac{\sqrt{\kappa_e}}{(\kappa/2 - i\Omega_m)^2} s_0 \quad (\text{S32})$$

The resulting microwave signal coming out of the cavity is an interference between the probe tone and the sideband at the same frequency and is calculated as

$$S_{11} = 1 - \frac{\kappa_e}{\kappa/2 - i\Omega_m} + C \frac{\kappa\kappa_e/2}{(\kappa/2 - i\Omega_m)^2} \quad (\text{S33})$$

#### 5. Amplification for $\Omega = -\Omega_m$

When we probe on the red side of the drive, the physical mechanisms are essentially identical to the blue detuned probe. We get

$$a_- = \frac{\sqrt{\kappa_e}}{\kappa/2 + i\Omega_m} s_0 + \frac{\kappa}{2} C \frac{\sqrt{\kappa_e}}{(\kappa/2 + i\Omega_m)^2} s_0 \quad (\text{S34})$$

and

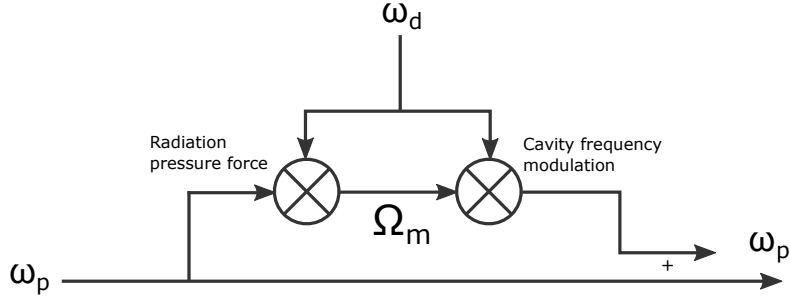

FIG. S4. (a) A circuit diagram interpretation of the amplification mechanism. The amplification can be viewed as the effect of two frequency mixers – one which corresponds to the driving of the mechanics by the beating of the probe  $\omega_p$  and drive  $\omega_d$ , and one which is caused by the mechanical modulation of the cavity frequency. The result of the last mixing step creates sidebands of the drive tone, one of which interferes with the probe tone.

$$S_{11} = 1 - \frac{\kappa_e}{\kappa/2 + i\Omega_m} - C \frac{\kappa\kappa_e/2}{(\kappa/2 + i\Omega_m)^2}. \quad (\text{S35})$$

## S6. DOUBLE MIXER AMPLIFICATION

The amplification mechanism can be understood as a frequency mixing circuit as depicted in Fig. S4. Note that this assumes that there are no dynamical effects, as this model is most accurate when the drive tone is at the center of the cavity frequency. There are two frequency mixing steps in this optomechanical amplifier. First, the probe and drive tone interfere and beat at their difference frequency, which is the same as the mechanical frequency  $\Omega_m$ . Due to the radiation pressure force, the mechanical resonator is coherently driven by the amplitude modulations. The mechanical resonator is also coupled to the cavity frequency, and the cavity response will oscillate. Since the drive tone is tuned to the center, it will only experience phase modulation, the magnitude of this being proportional to the slope of the cavity phase response at the center frequency. The sidebands then created from the drive tone are of equal magnitude, but opposite phase, and thus interfere with the probe tone in opposite directions, as shown in the last term of Eq. (S20). This effect is visually shown in Fig. S5. When the magnitude of the sidebands are smaller than the magnitude of the

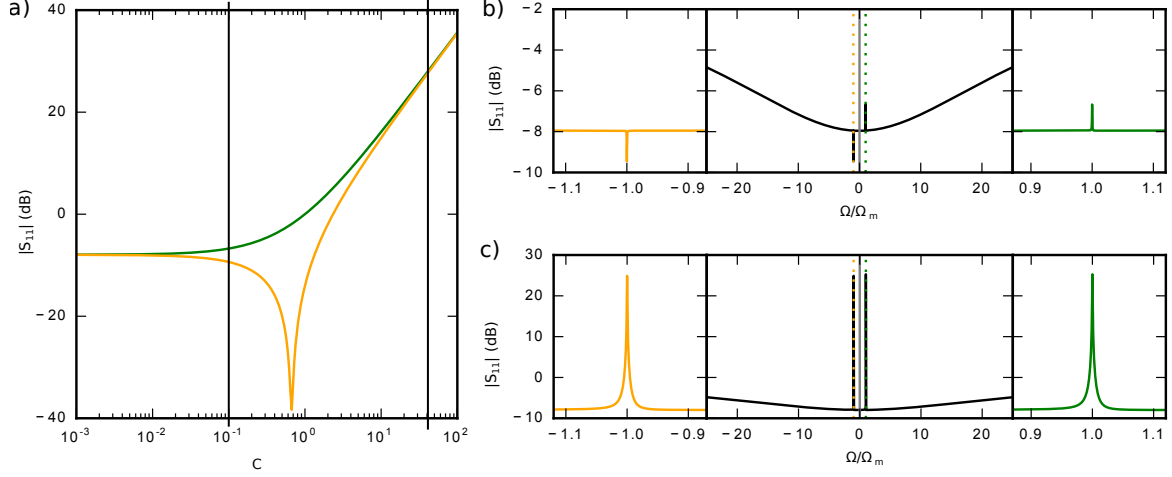

FIG. S5. (a) The trend of the magnitude of the reflection coefficient of the sidebands, depending on the multi-photon cooperativity. The parameters we chose are for an undercoupled cavity  $\eta = 0.3$  and a highly sideband unresolved cavity  $\Omega_m/\kappa = 0.01$ . The green curve corresponds to  $\Omega = +\Omega_m$  and the yellow curve corresponds to  $\Omega = -\Omega_m$ . There are two linecuts in the figure, one at  $C = 0.1$ , which is further shown in (b) and another at  $C = 30$  which is shown in (c). (b)-(c) Are linecuts where we show the entire cavity response in the center and zoom-ins of the upper (green) and lower (yellow) sidebands on the sides.

reflected probe tone, one can see in Fig. S5(b) that the interference is destructive for the lower sideband and constructive for the upper sideband. Note that this effect is exactly the opposite for the upper and lower sidebands when the cavity is overcoupled such that the slope of the phase is equal but opposite in sign. When the pump power is increased such that the sidebands are of a far greater magnitude than the reflected probe tone, it overpowers the probe tone and both detunings converge to the same high gain value in magnitude.

## S7. INTUITION BEHIND QUANTUM-LIMITED AMPLIFICATION

An amplifier is said to be quantum limited if the dominant cause of noise in the amplified signal is due to quantum processes instead of thermal noise. Fig. S6 gives a diagrammatic explanation of how our system would allow quantum-limited amplification provided the drive tone is strong enough. Thermal noise of the mechanical mode is a Lorentzian distribution in the power spectral density centered around the mechanical resonance frequency where the

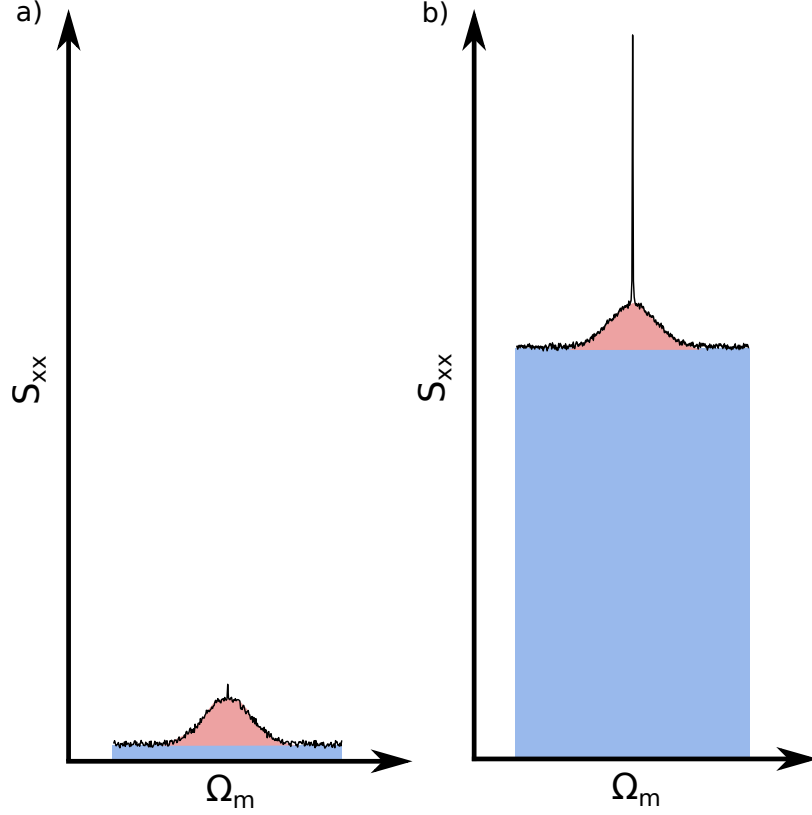

FIG. S6. A schematical description of how quantum-limited amplification is possible in this optomechanical system. Both graphs show the power spectral density of the mechanical oscillator and are a combination the quantum noise floor (blue area), thermal noise (red area) and a delta peak which is driven by the beating of the pump and probe. (a) At low pump power, the thermal noise is quit large compared to the quantum noise floor. (b) At high powers, both the delta peak and noise floor are increased in magnitude, but the thermal noise stays the same. Taken to sufficiently high powers, the thermal noise is insignificant compared to the quantum noise.

area is proportional to the average number of phonons. Coherently driving this mode using the beating of the probe and pump tone will excite a delta peak inside of the Lorentzian profile, as seen in Fig. S6. The important part is that no matter how strong the drive tone is, the thermal peak will stay the same size, while the delta peak will increase. Furthermore, the probe tone will inevitably have a small frequency-independent quantum noise floor, indicated by the dotted lines. Once the power is sufficient such that the thermal noise is proportionally insignificant to the amplified quantum noise, the amplification is said to be quantum-limited.

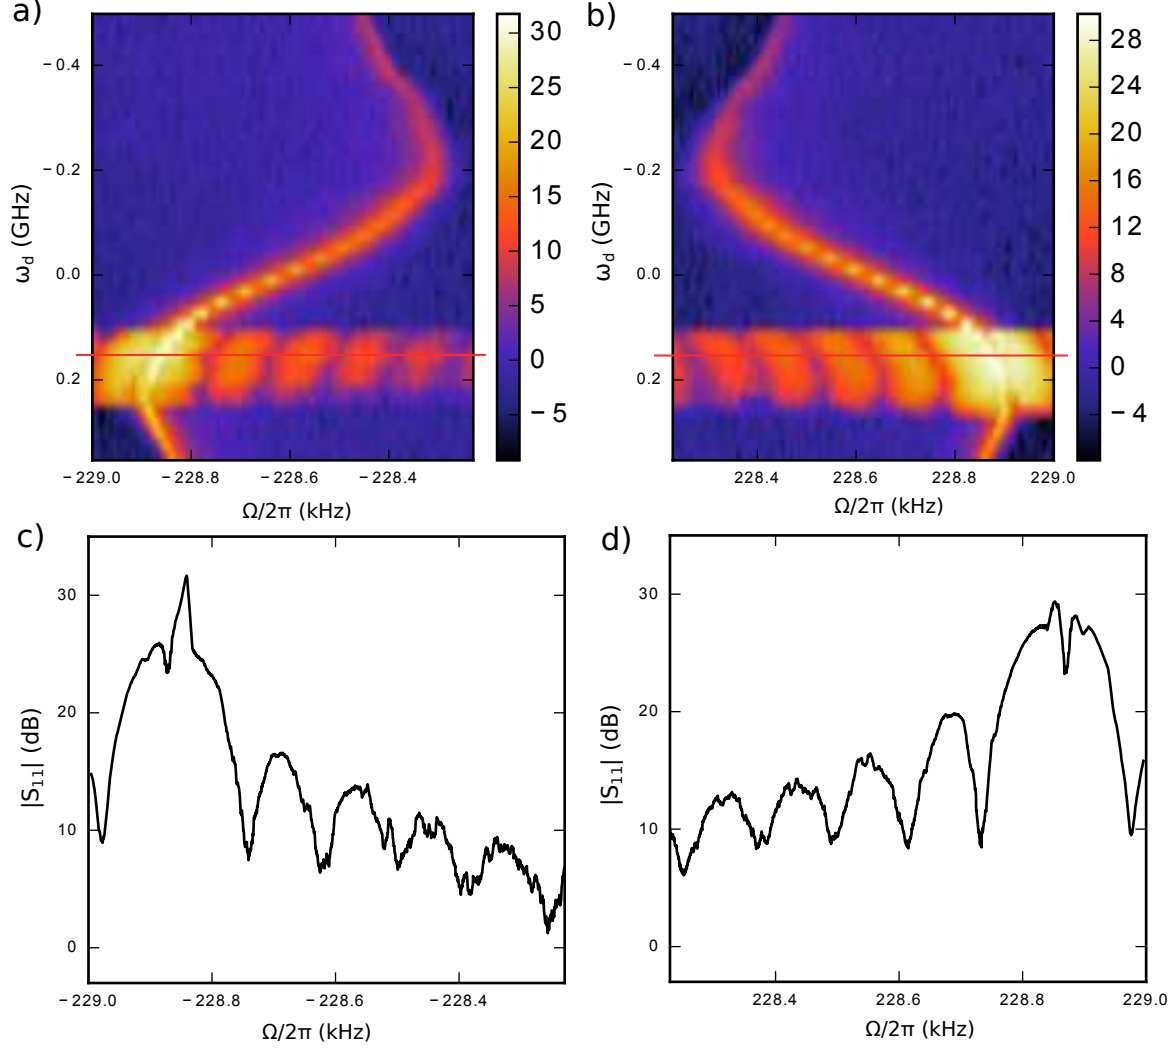

FIG. S7. A 2D plot showing the magnitude of the reflection coefficient with respect to the drive tone and the probe detuning around  $\Omega \sim -\Omega_m$  (a) and  $\Omega \sim +\Omega_m$  (b) at 7 dBm input power at the cavity. The optical spring effect is expressed as a detuning-dependent mechanical frequency. However, when the drive detuning is positively detuned, we see an artifact which seems to be self-oscillations. The red line in (a) corresponds to the linecut taken for (c). Likewise, the red line in (b) is plotted in (d).

## S8. OPTICAL SPRING EFFECT

We detune the drive tone from the cavity resonance and observe the optical spring effect<sup>S4</sup> – a mechanical spring constant, hence also frequency, that is dependent on the drive detuning – in both the upper and lower sidebands of the OMIR signal. We observe a deviation which

spans 580 Hz which is  $\approx 27\Gamma_m$ . A byproduct of optical damping is that one can decrease the mechanical linewidth to such an extent that the effective loss rate becomes negative, indicating self-oscillations, which can be seen for our system in Fig. S7(c)-(d) for both negative and positive probe detunings. The measurement takes the shape of a Fraunhofer diffraction pattern when we sweep the probe tone of the vector network analyzer.

- 
- [S1] P.-L. Yu, T. Purdy, and C. Regal, Physical review letters **108**, 083603 (2012).
  - [S2] S. Weis, R. Rivière, S. Deléglise, E. Gavartin, O. Arcizet, A. Schliesser, and T. J. Kippenberg, Science **330**, 1520 (2010).
  - [S3] M. Aspelmeyer, T. J. Kippenberg, and F. Marquardt, Reviews of Modern Physics **86**, 1391 (2014).
  - [S4] M. Hossein-Zadeh and K. J. Vahala, Optics letters **32**, 1611 (2007).
